# Supplementary material for: Semantic Term "Blurring" and Stochastic "Barcoding" for Improved Unsupervised Text Classification
Source: arXiv:1811.02456 source file (2018-11-06)
Supplement: Supplementary file 1 [file appendix.tex]

/chapter{Appendix}
